# Supplementary material for: CARZero: Cross-Attention Alignment for Radiology Zero-Shot Classification
Source: arXiv:2402.17417 source file (2024-03-24)
Supplement: Supplementary file 1 [file X_suppl.tex]

\clearpage
\appendix
\setcounter{page}{1}
\maketitlesupplementary

\section{Comparison with State-of-the-art Methods}
\label{sec:add_comparision}

% 我们展示了本文方法与现有sota的 image-text pretraining方法对比在不同数据上的详细结果 under zero-shot classification.Figure x 展示了openi数据. Table X展示了CheXray14数据集. Table X展示了CheXpert数据集.  Table X展示了ChestDet10数据集. FigureX~XI展示了padchest数据集的结果. Figure XII-XIII展示了CARZero和MedKLIP的可视化对比结果,可以发现我们提出的CARZero能更准确的捕捉到疾病在CXR中的对应位置. Figure XIIII展示了CARzero中的Similarty representation的t-sne可视化结果.首先从Figure XIIII (a)中可以发现,相同类别的SimR都被聚成一类,而不同类别的SimR是完全分开的.这证实了本文提出的图像和文本的SimR能够有效对齐图像和文本的空间.接着,Figure XIIII (b)-(f)中可以发现,我们得到的SimR是一种 reasonable disease-level semantic information.

In this section, we present a detailed comparison of our proposed \algname with the existing state-of-the-art (SOTA) image-text pretraining methods in various datasets under zero-shot classification settings.

\Cref{fig:openi} illustrates the results obtained on the Open-I dataset. This results demonstrate the efficacy of our method in discerning distinct disease categories, showcasing our approach's robust performance in comparison to existing methodologies.

\Cref{tab:chexray14}, \Cref{tab:chexpert}, and \Cref{tab:chestxdet10} respectively present the comprehensive results on the CheXray14, CheXpert, and ChestDet10 datasets. These tables offer a detailed quantitative analysis, highlighting the superior diagnostic performance and consistency of our method across a wide range of medical conditions.

\Cref{fig:padchest_0_64}, \Cref{fig:padchest_64_128}, and \Cref{fig:padchest_128_192} encompass the results on the PadChest dataset. The figures provide an insightful view into the performance of our method, detailing how our method effectively handles the dataset's extensive variety of chest X-rays and intricate classifications.

\section{Additional Visualization Results}
\label{sec:add_visualization}
In this section, we delve deeper into the visualization aspects of our study, focusing on the comparative and analytical visual representations that further substantiate the effectiveness of our proposed method. These additional visualizations not only provide empirical evidence supporting our model's superiority in various scenarios but also offer intuitive insights into the intricate workings of the model. By presenting these results, we aim to offer a more comprehensive understanding of how our approach advances the field of zero-shot learning in medical image analysis.

\Cref{fig:visual_complete} and \Cref{fig:visual_complete_rest} offer a comparative visualization between our proposed \algname and MedKLIP. These figures elucidate how \algname more accurately captures the corresponding locations of diseases in CXR images. The precision in identifying disease-specific regions underscores the advanced capabilities of \algname in medical image analysis.

\Cref{fig:tsne} showcases the t-SNE visualization of Similarity Representations (SimR) within \algname. \Cref{fig:tsne:sub1} reveals a distinct clustering of SimRs within the same categories, while ensuring clear separation among different categories. This observation confirms the effectiveness of our proposed SimR in aligning the image and text spaces accurately. Subsequently, \Cref{fig:tsne:sub2} to \Cref{fig:tsne:sub6} demonstrate that the SimR we obtained carry reasonable disease-level semantic information. This aspect highlights our method's nuanced understanding and representation of medical conditions at a semantic level, further validating the practical utility of our approach in clinical settings.

\begin{figure*}[b]
  \centering
    \includegraphics[width=0.95\linewidth]{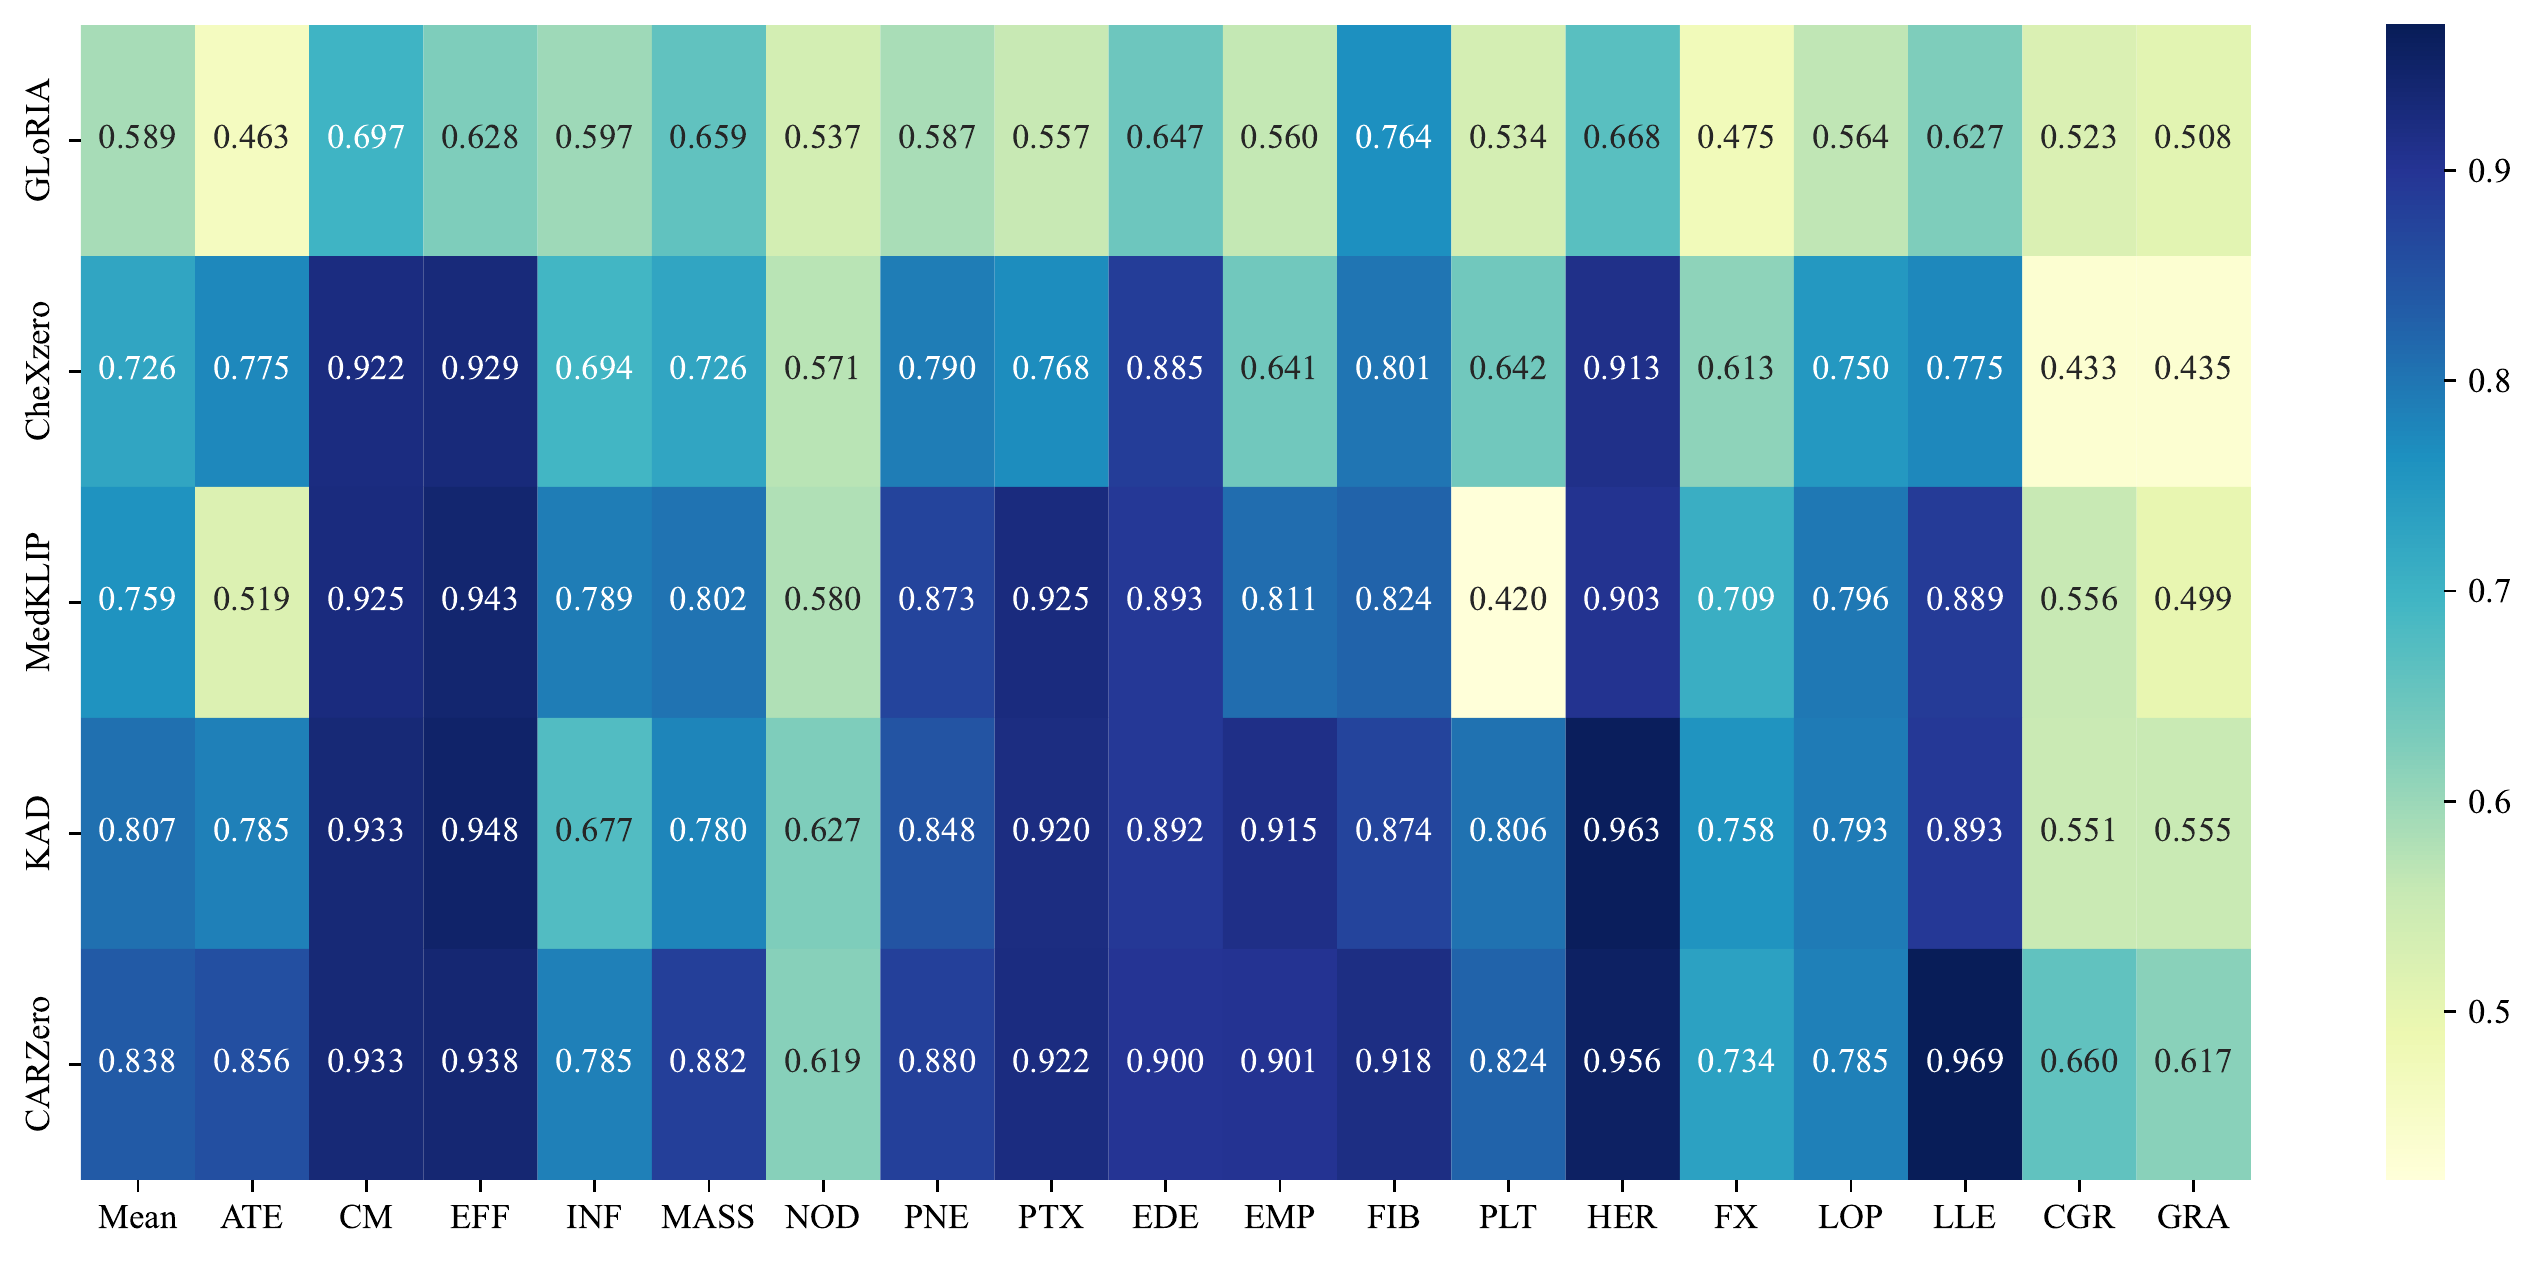}
    \caption{Comparative analysis between the existing zero-shot classification approaches and our proposed \algname method, applied to Open-I dataset across 18 disease categories in terms of AUC performance. The abbreviations ATE, CM, EFF, INF, MASS, NOD, PNE, PTX, EDE, EMP, FIB, PLT, HER, FX, LOP, LLE, CGR, and GRA correspond to Atelectases, Cardiomegaly, Effusion, Infiltrate, Mass, Nodule, Pneumonia, Pneumothorax, Edema, Emphysema, Fibrosis, Pleural Thickening, Hernia, Fracture, Lung Opacity, Lung Lesion, Calcified Granuloma, and Granuloma, respectively.} 
    % \vspace{-1mm}
    \label{fig:openi}
    % \vspace{-4mm}
\end{figure*}

\begin{figure*}[t]
  \centering
    \includegraphics[width=0.95\linewidth]{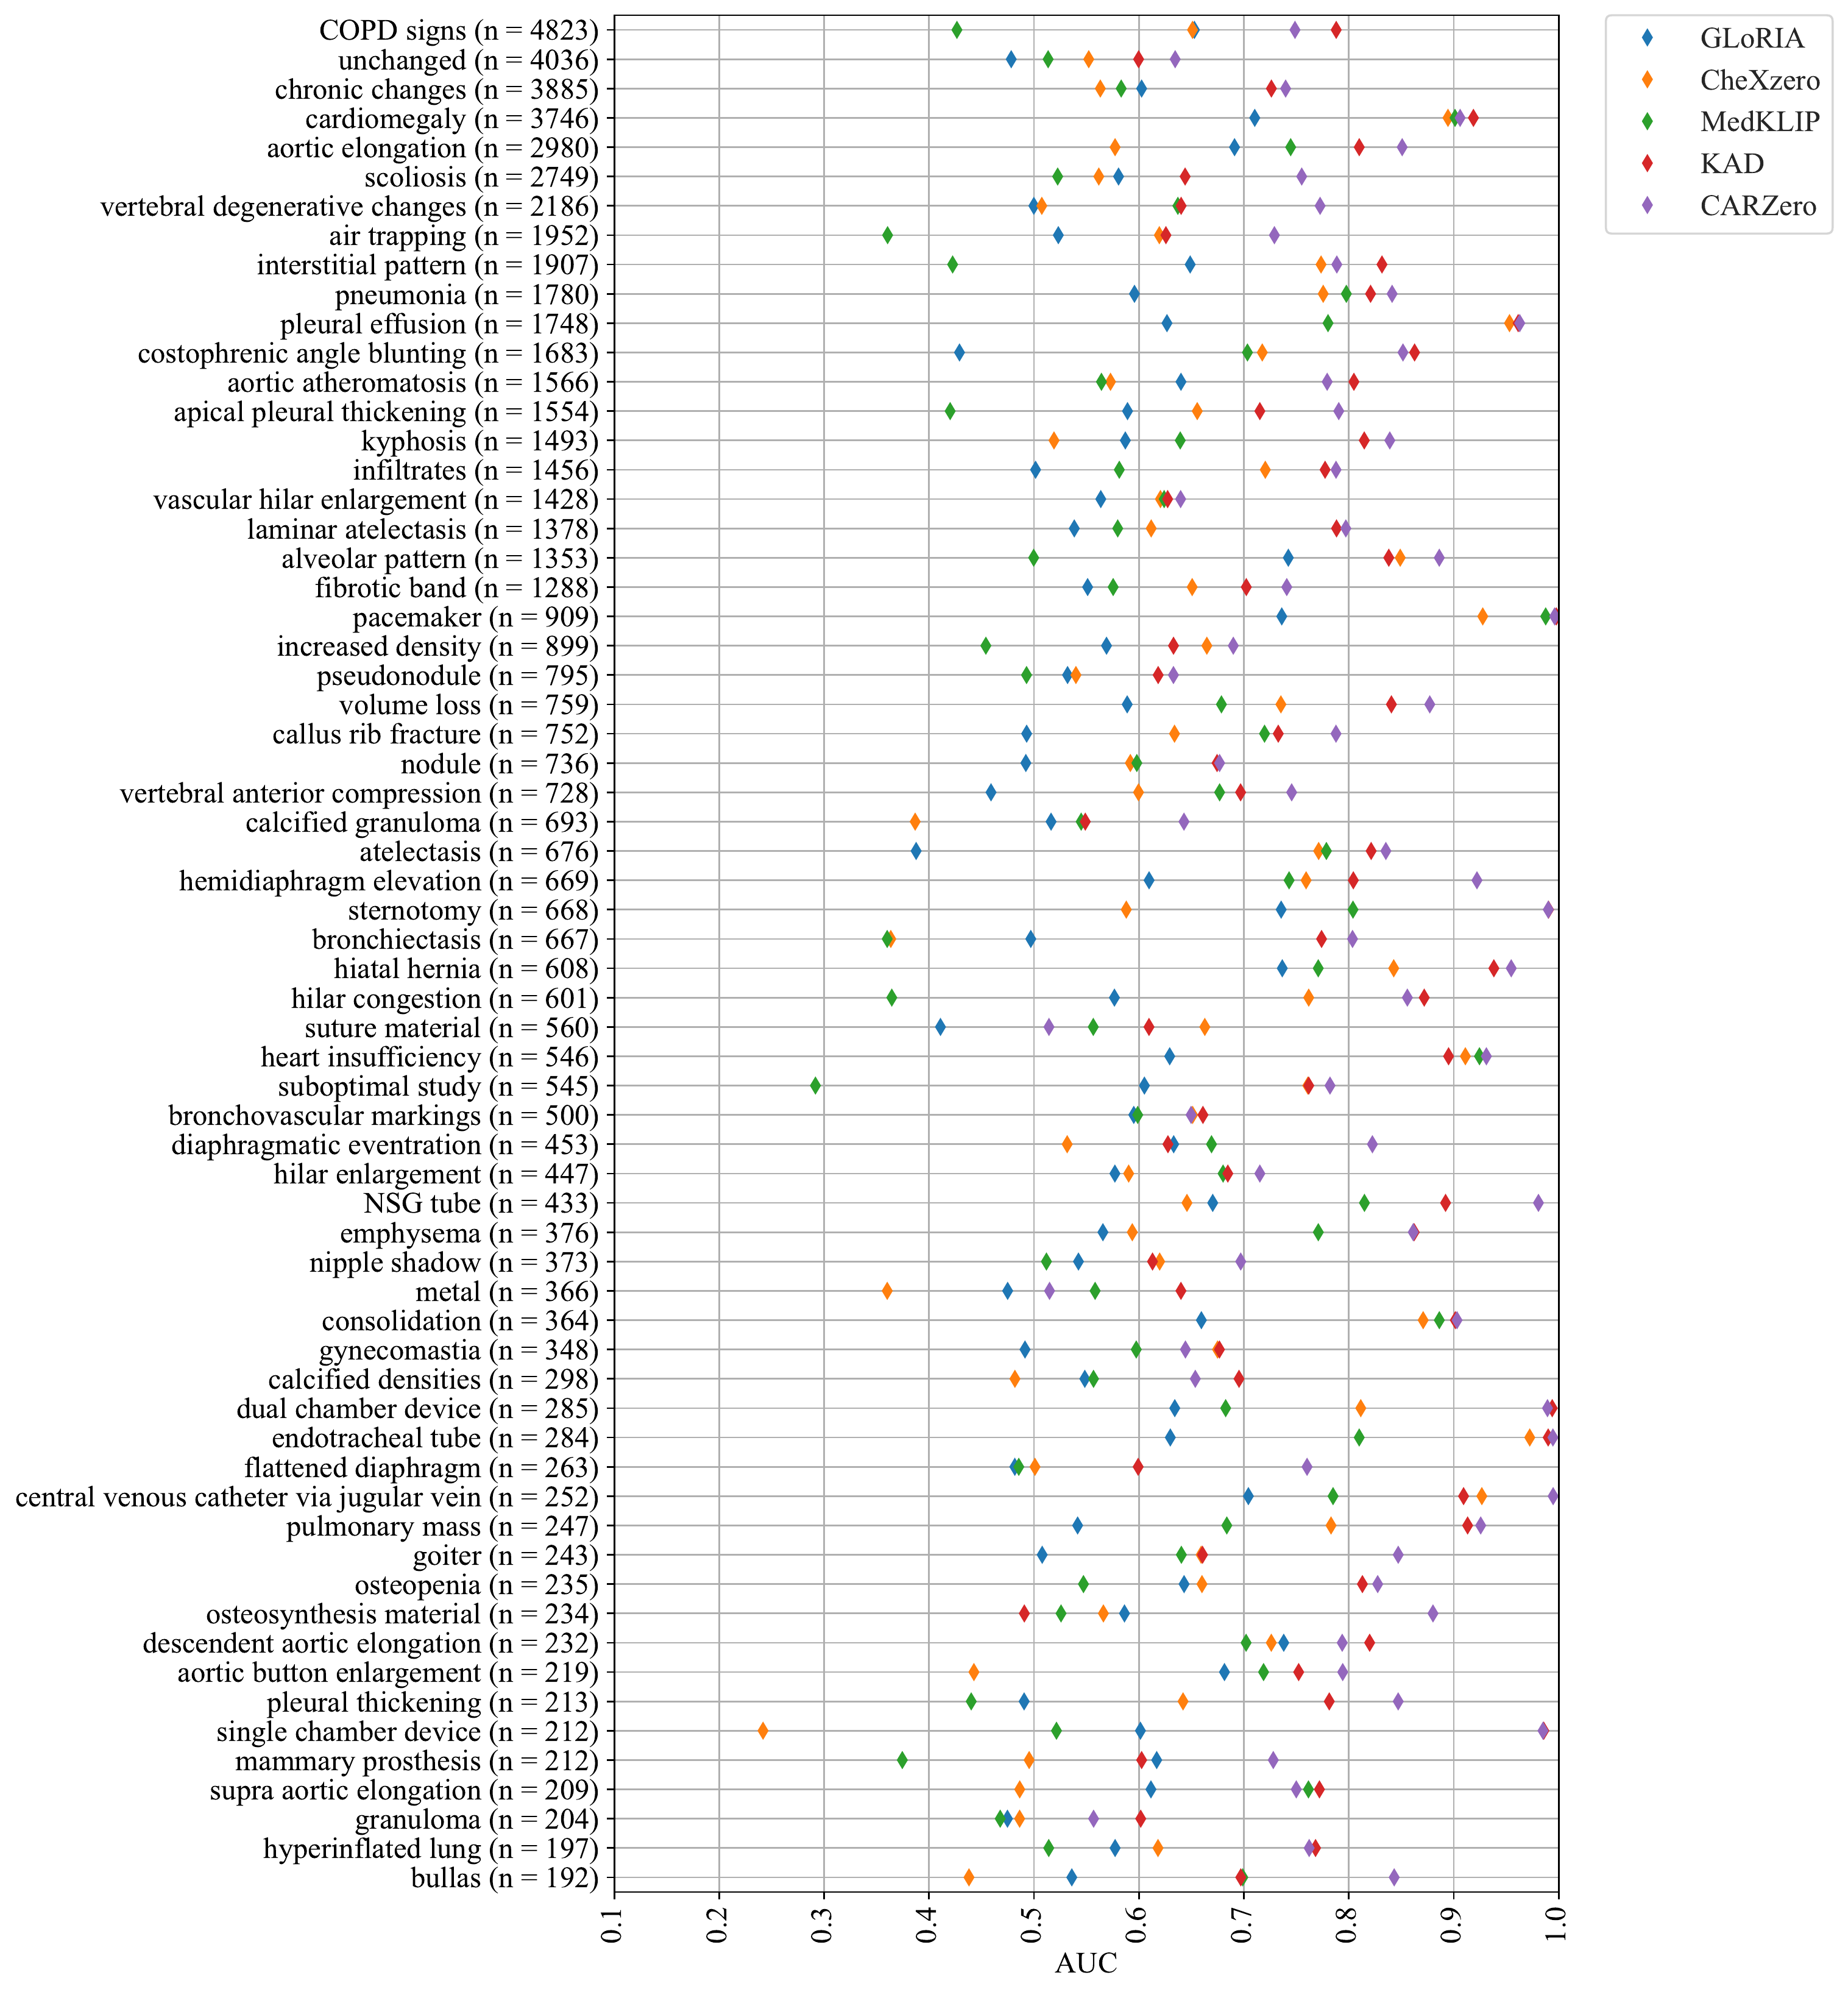}
    \caption{Comparative analysis between the existing zero-shot classification approaches and our proposed \algname method, applied to the human-annotated subset of the PadChest dataset (totalling 39,053 chest X-rays and 192 classes). The results for the \textbf{1-64} classes are shown here. Mean AUC are shown for each class, and $n$ refers to the number of positive samples.} 
    % \vspace{-1mm}
    \label{fig:padchest_0_64}
    % \vspace{-4mm}
\end{figure*}

\begin{figure*}[t]
  \centering
    \includegraphics[width=0.95\linewidth]{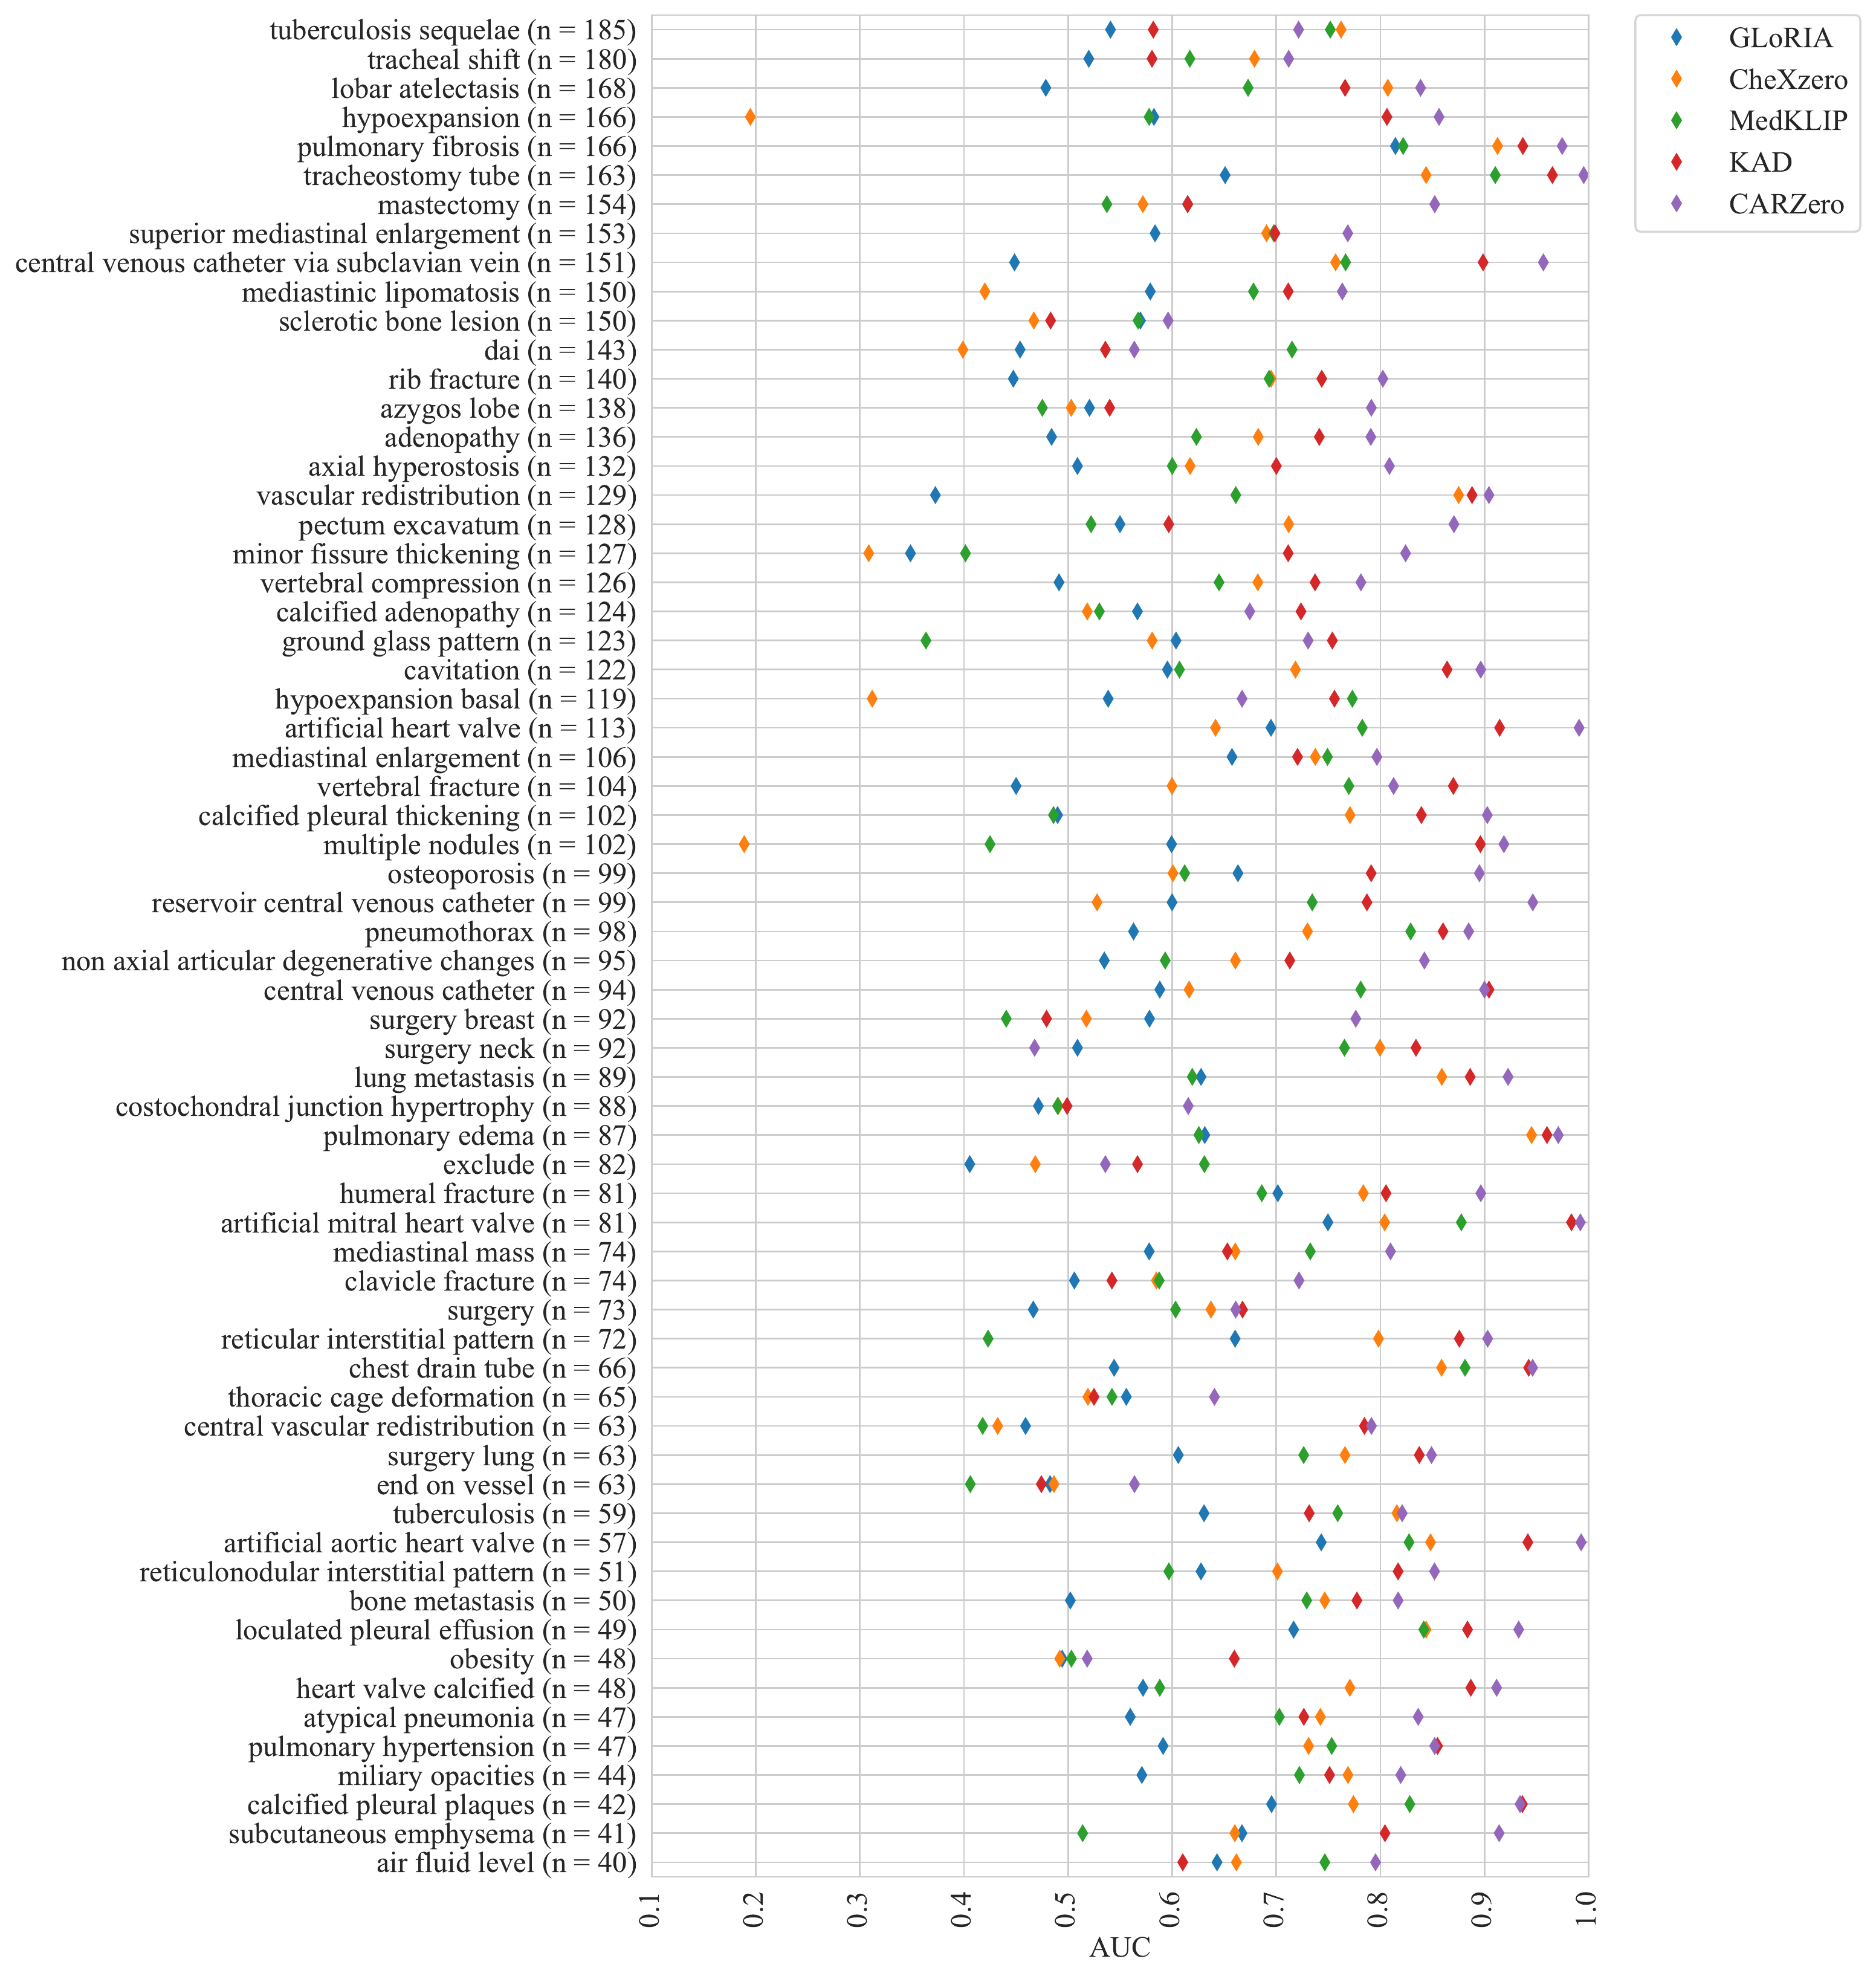}
    \caption{Comparative analysis between the existing zero-shot classification approaches and our proposed \algname method, applied to the human-annotated subset of the PadChest dataset (totalling 39,053 chest X-rays and 192 classes). The results for the \textbf{65-128} classes are shown here. Mean AUC are shown for each class, and $n$ refers to the number of positive samples.} 
    % \vspace{-1mm}
    \label{fig:padchest_64_128}
    % \vspace{-4mm}
\end{figure*}

\begin{figure*}[t]
  \centering
    \includegraphics[width=0.95\linewidth]{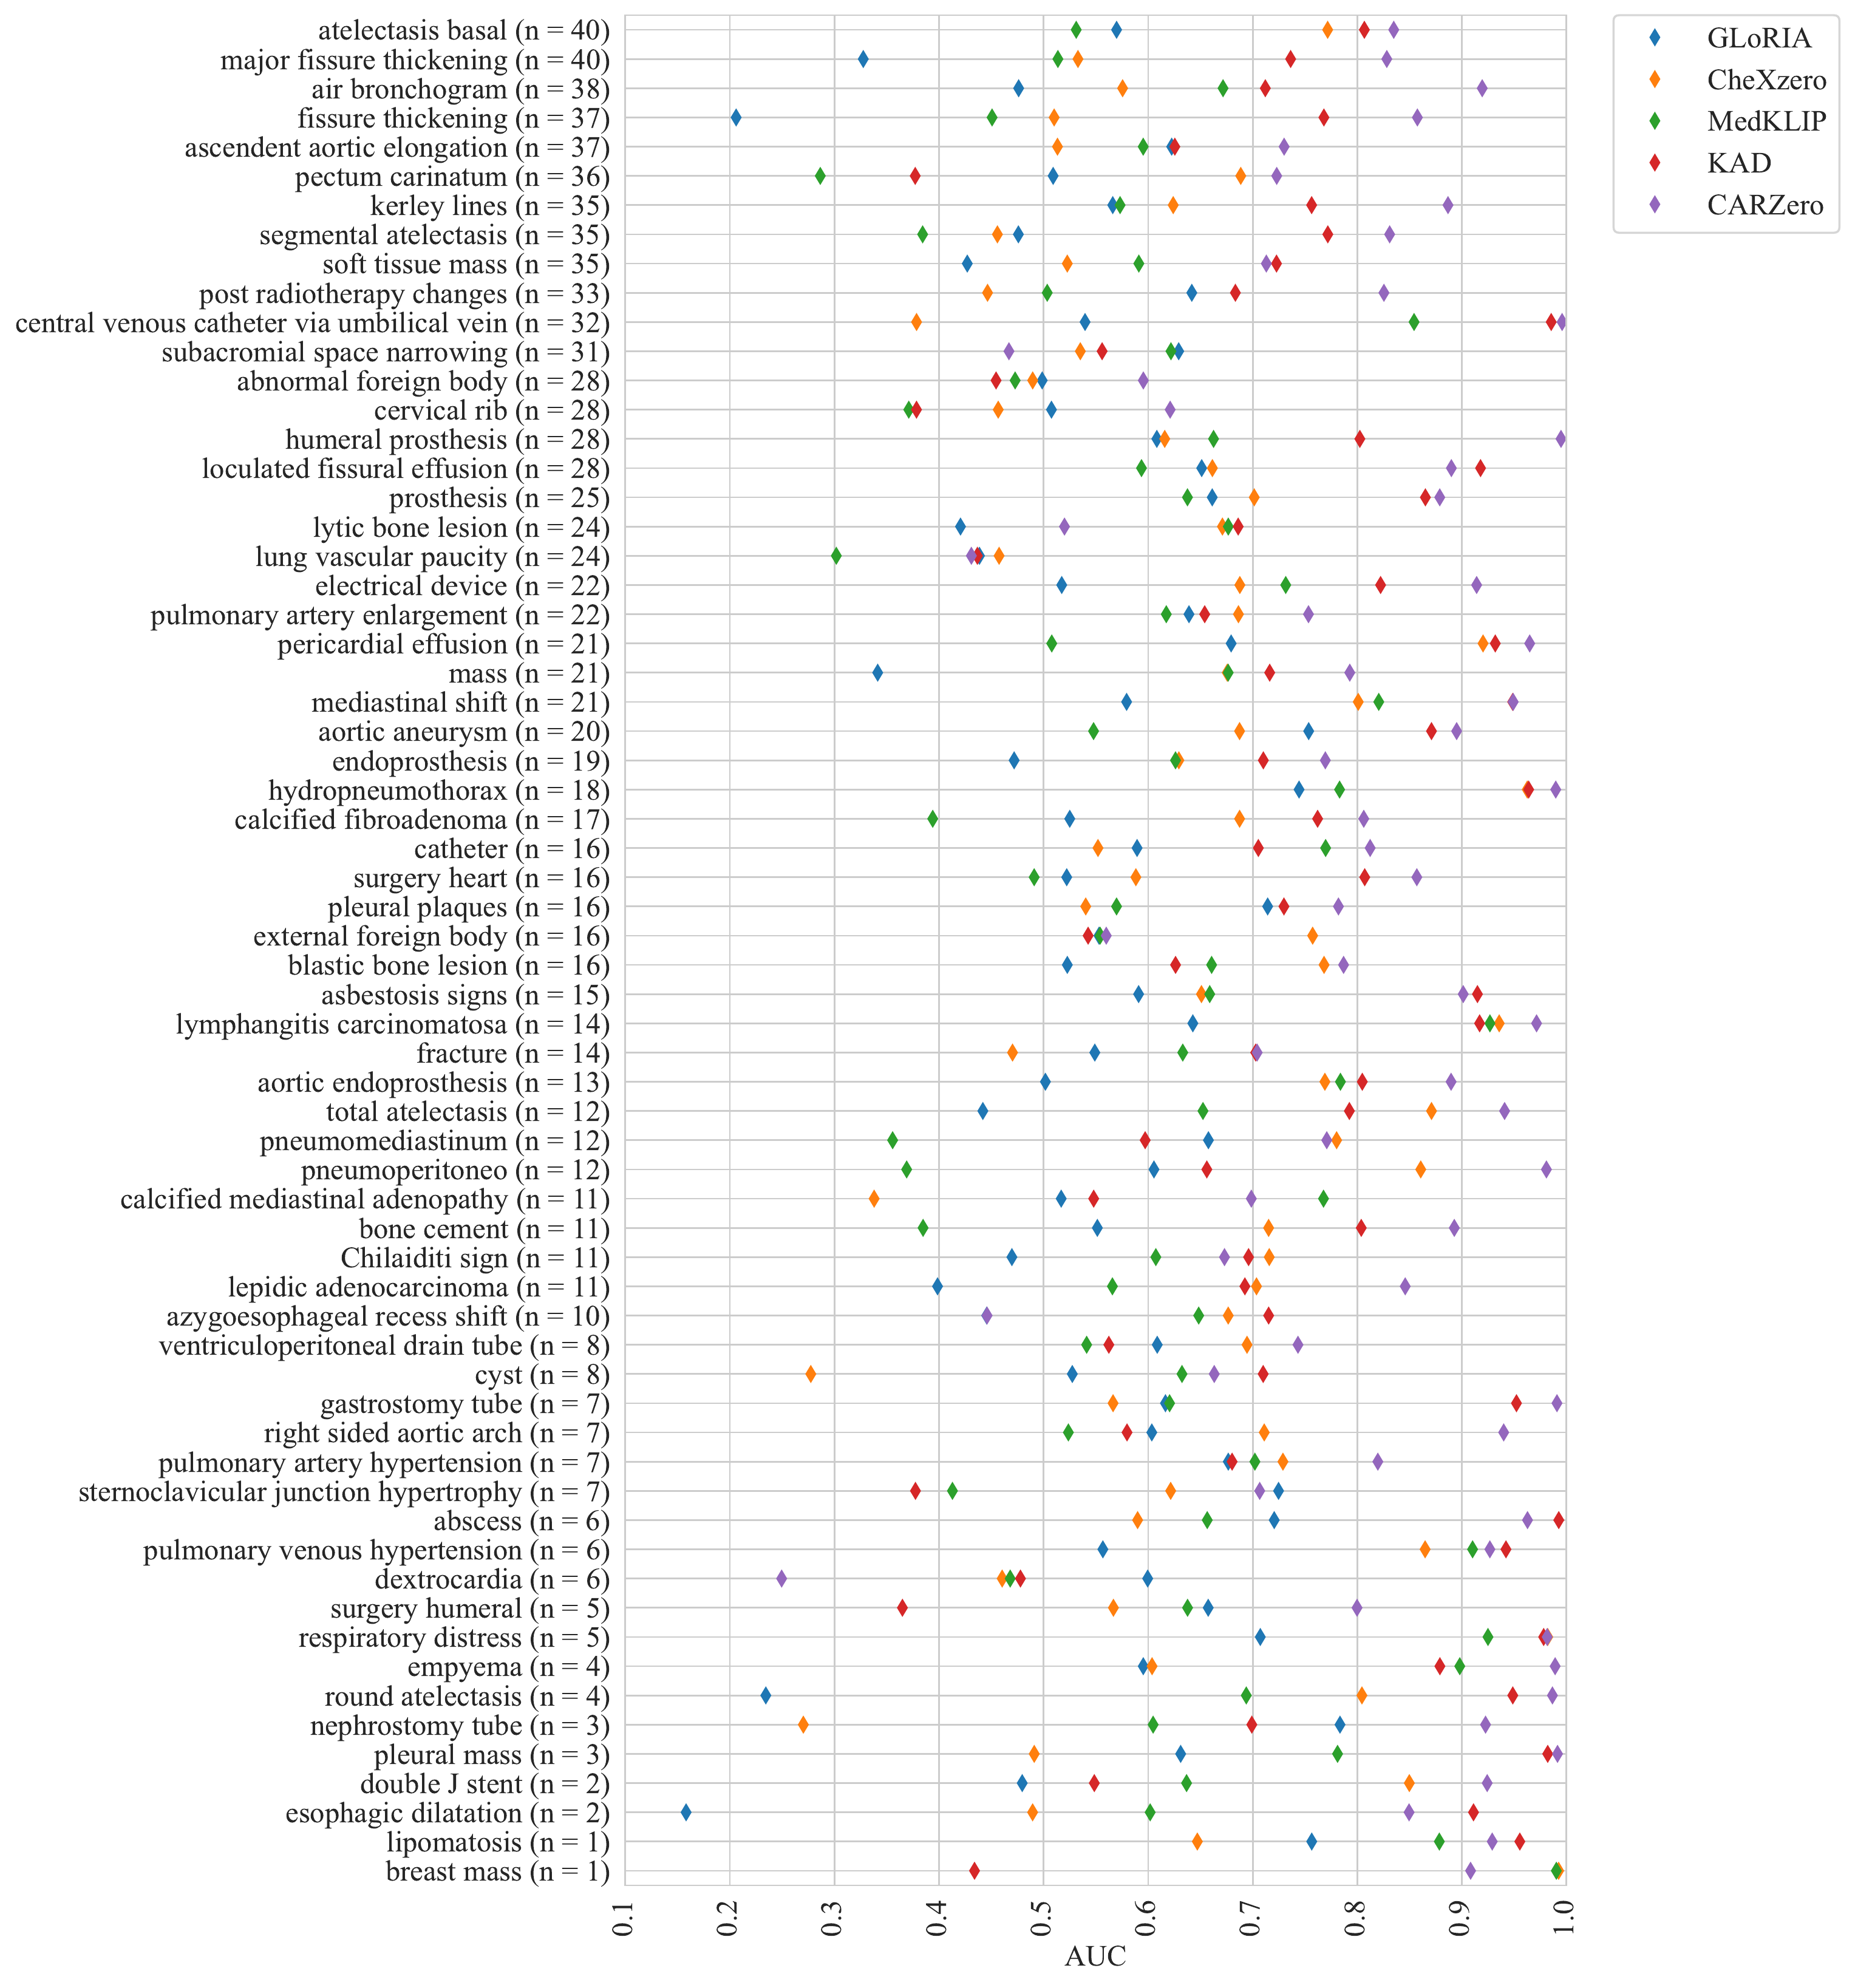}
    \caption{Comparative analysis between the existing zero-shot classification approaches and our proposed \algname method, applied to the human-annotated subset of the PadChest dataset (totalling 39,053 chest X-rays and 192 classes). The results for the \textbf{129-192} classes are shown here. Mean AUC are shown for each class, and $n$ refers to the number of positive samples.} 
    % \vspace{-1mm}
    \label{fig:padchest_128_192}
    % \vspace{-4mm}
\end{figure*}

\begin{figure*}[t]
  \centering
    \includegraphics[width=0.95\linewidth]{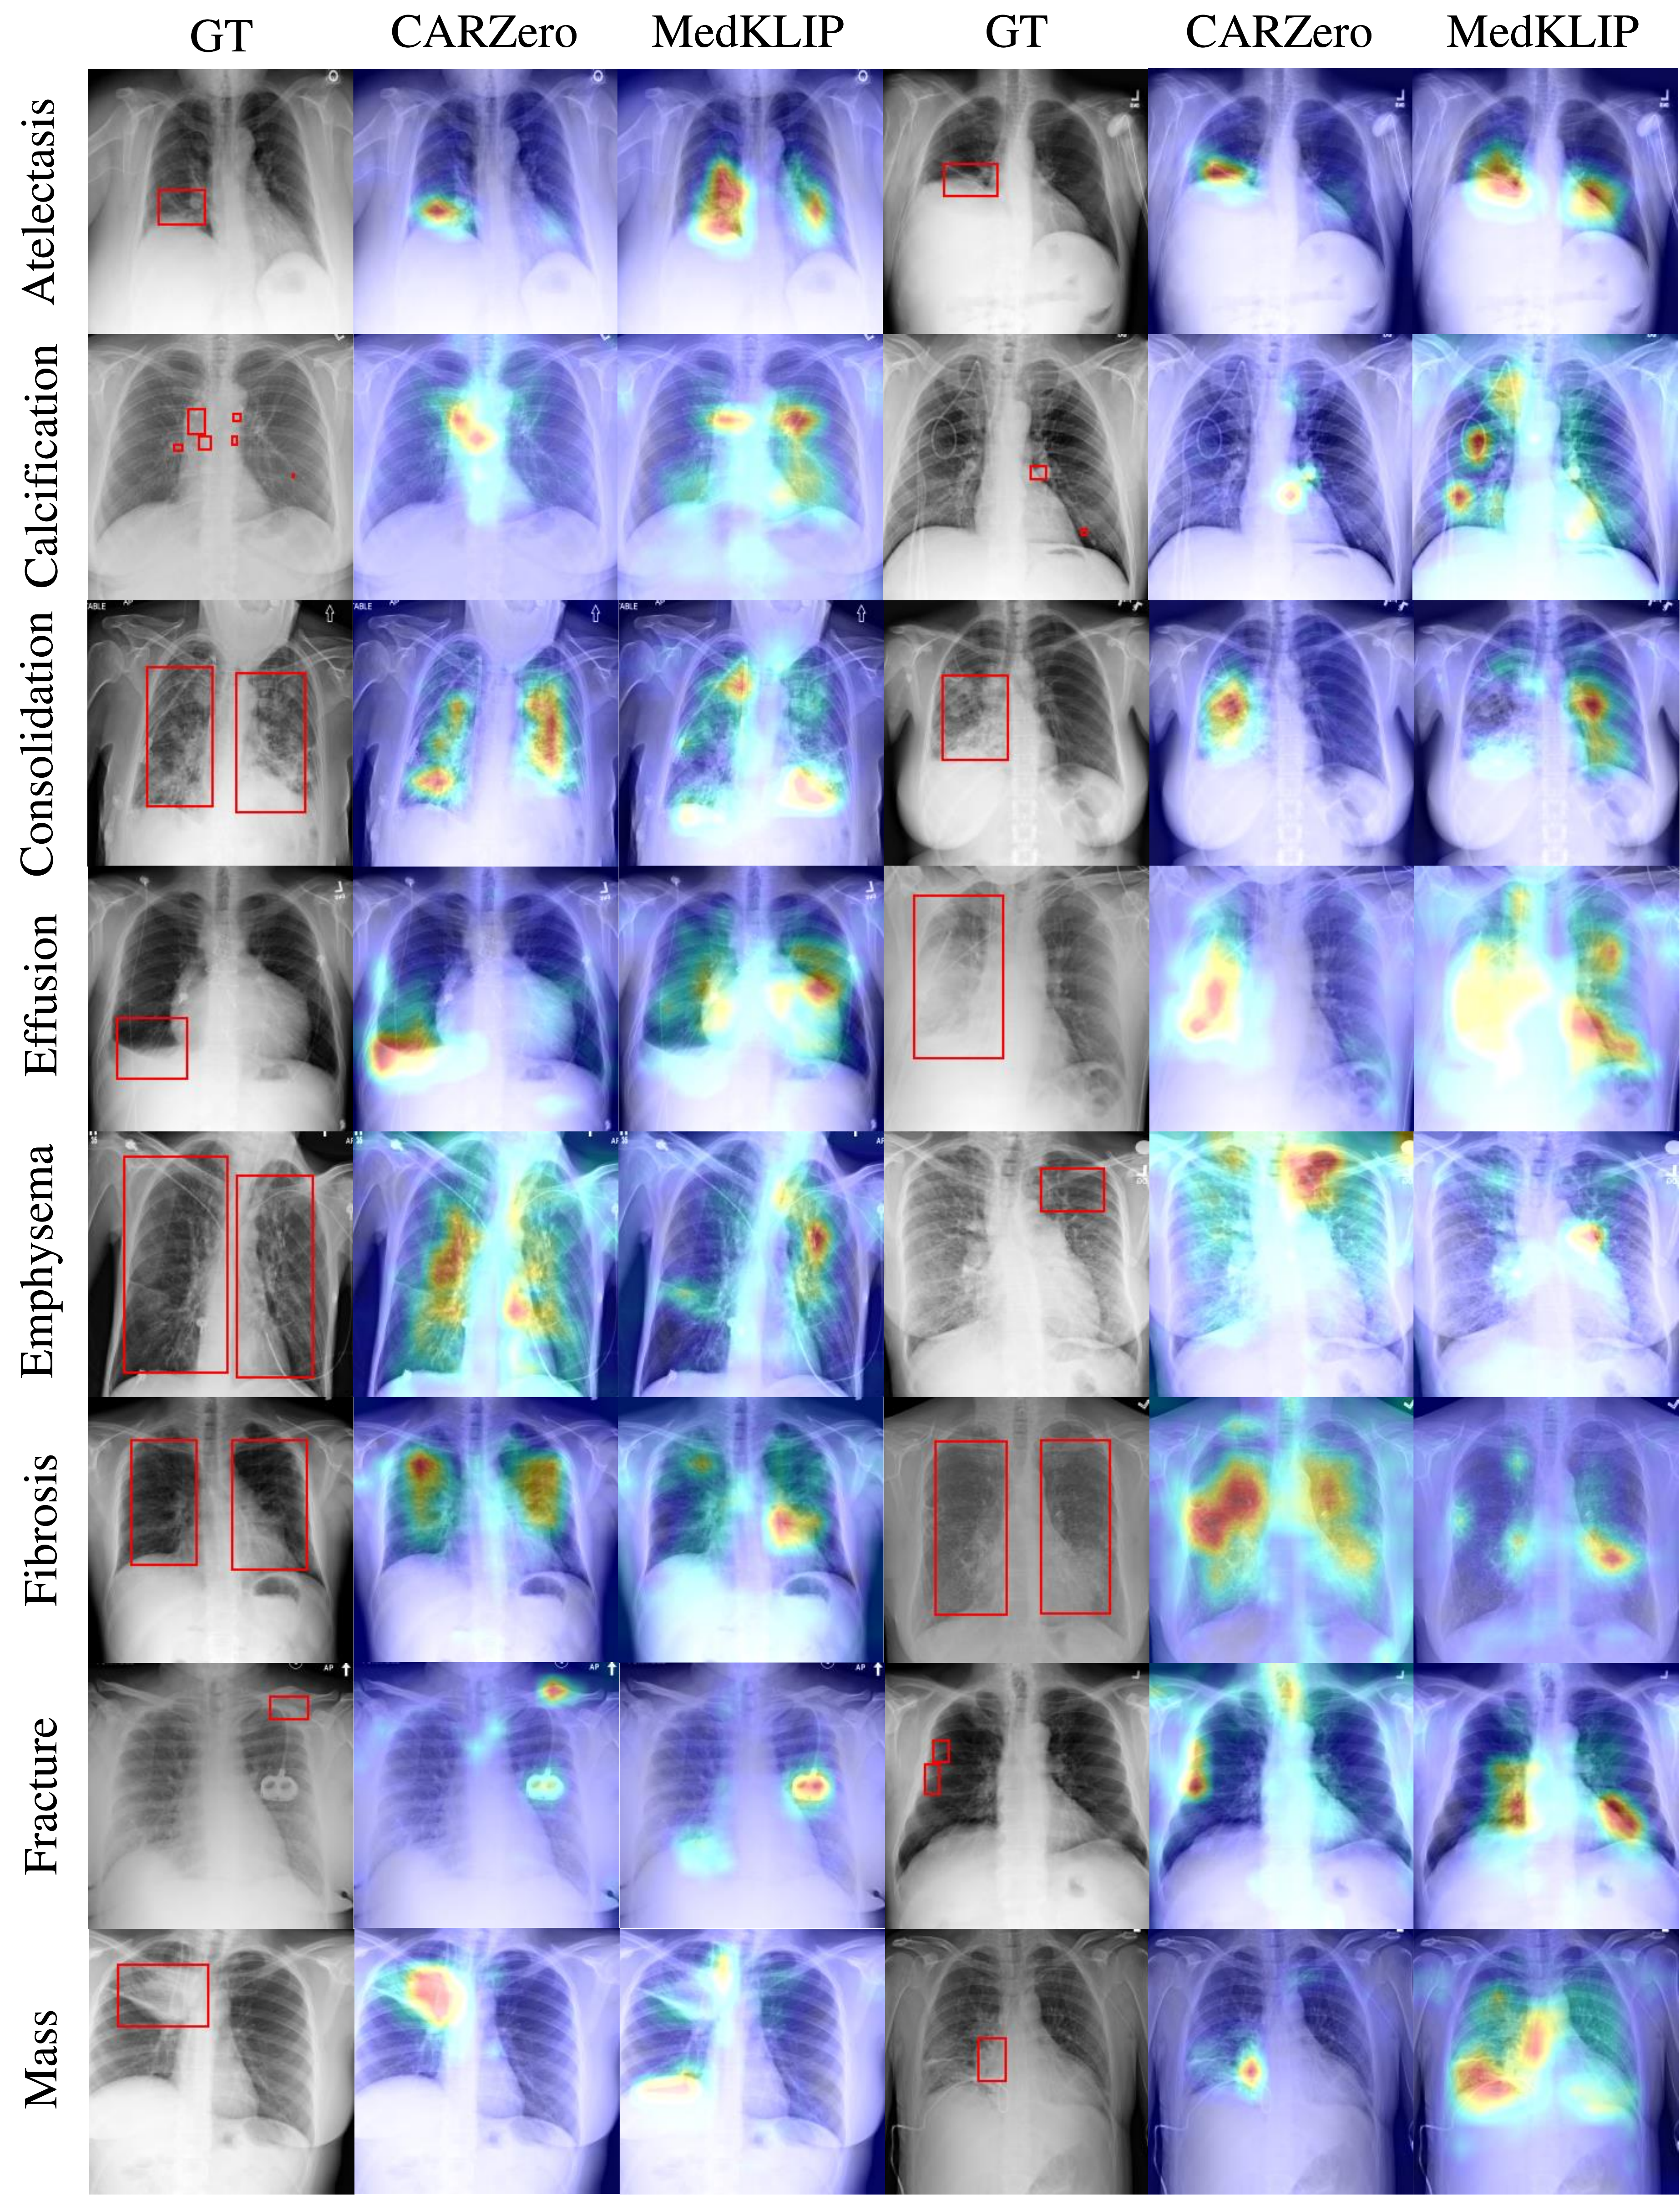}
    \caption{Comparative visualization of attention maps between \algname and MedKLIP on ChestXDet10 in a zero-shot Setting. This visualization displays the attention maps for classes \textbf{1-8}, where red boxes highlight the ground truth areas for detection. Areas with higher activation weights, indicating stronger correlations between specific words and image regions, are represented by highlighted pixels.} 
    % \vspace{-1mm}
    \label{fig:visual_complete}
    % \vspace{-4mm}
\end{figure*}

\begin{figure*}[t]
  \centering
    \includegraphics[width=0.95\linewidth]{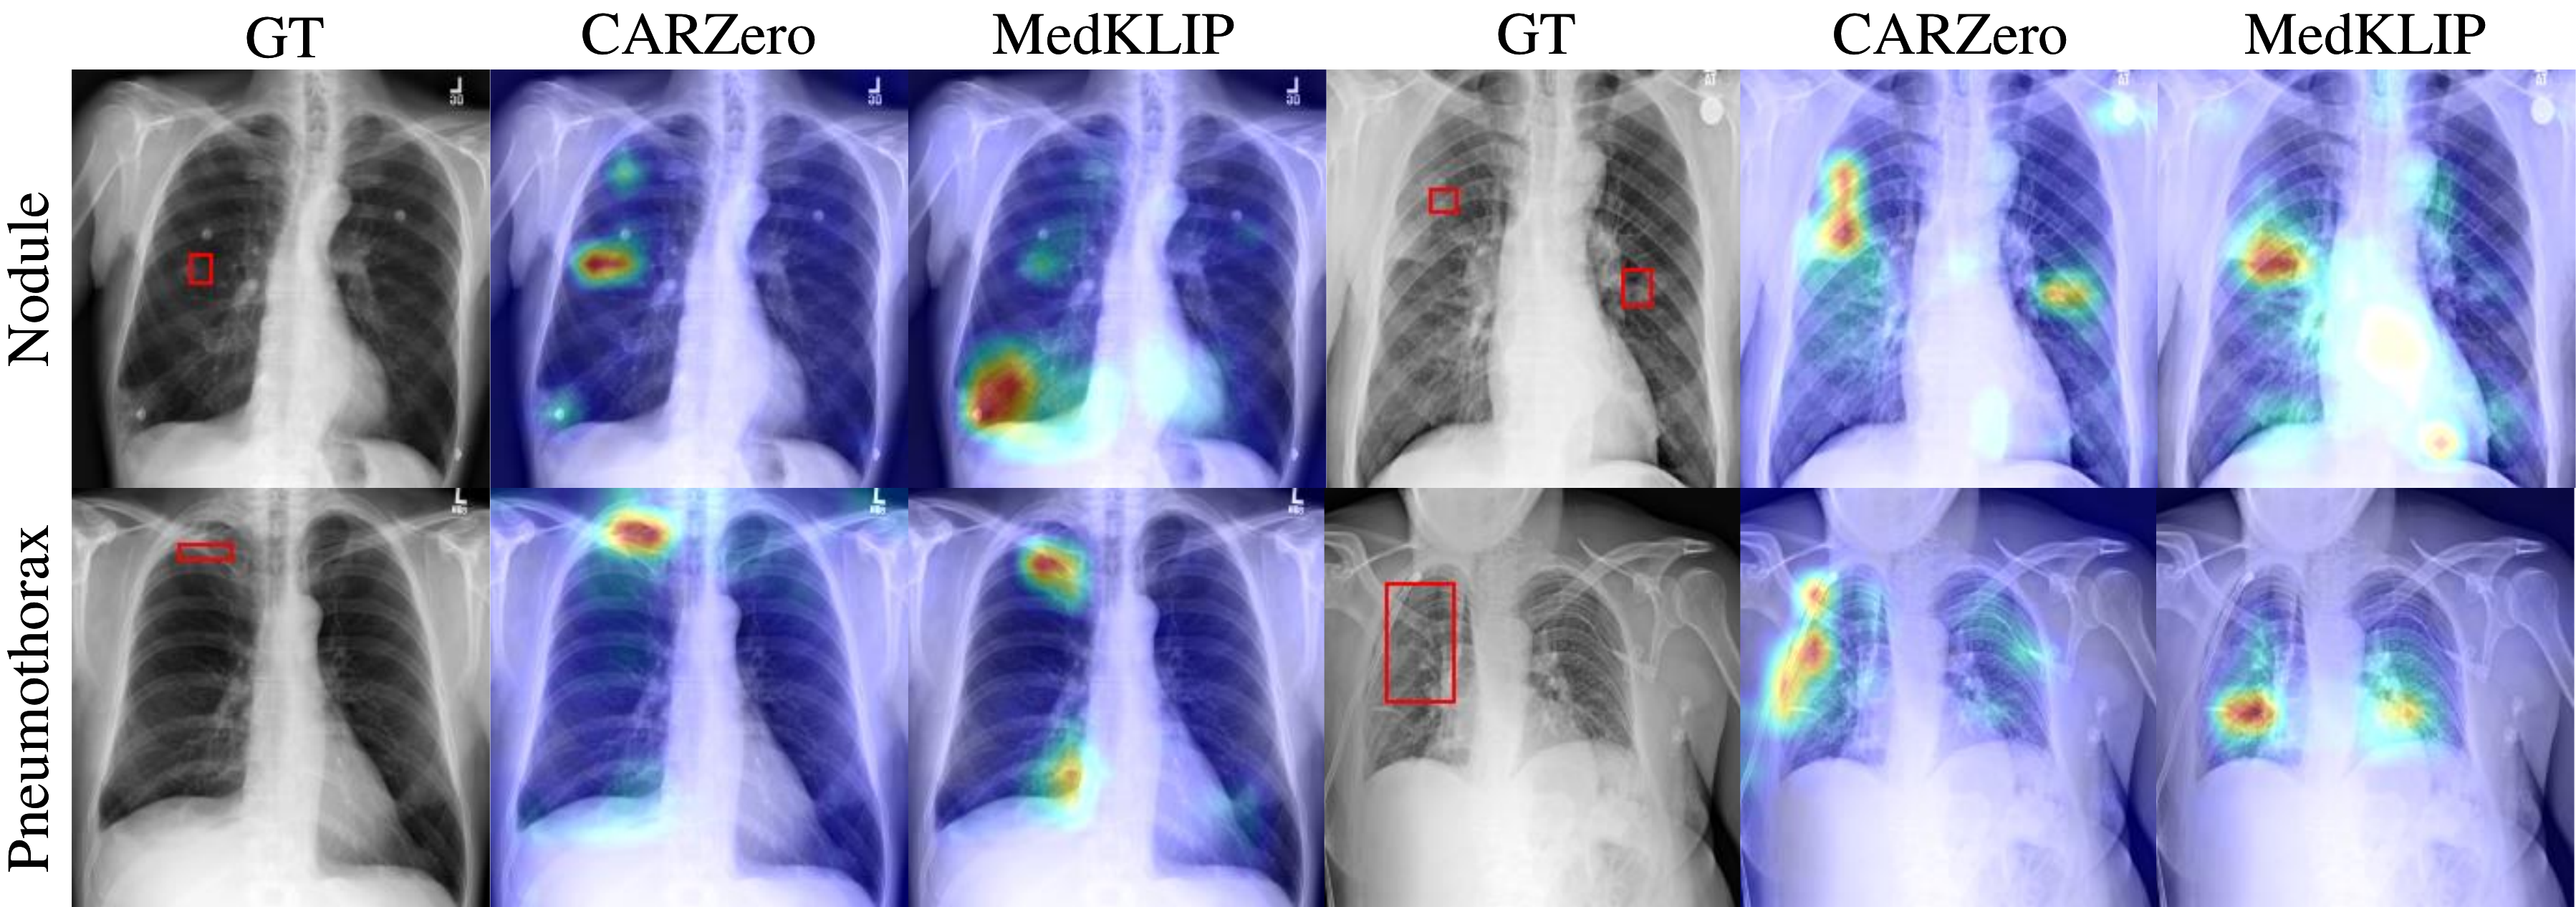}
    \caption{Comparative visualization of attention maps between \algname and MedKLIP on ChestXDet10 in a zero-shot Setting. This visualization displays the attention maps for classes \textbf{9-10}, where red boxes highlight the ground truth areas for detection. Areas with higher activation weights, indicating stronger correlations between specific words and image regions, are represented by highlighted pixels.} 
    % \vspace{-1mm}
    \label{fig:visual_complete_rest}
    % \vspace{-4mm}
\end{figure*}

\begin{table*}
  \centering
  \begin{tabular}{@{}l@{\hspace{7pt}}c@{\hspace{7pt}}c@{\hspace{7pt}}c@{\hspace{7pt}}c@{\hspace{7pt}}c@{\hspace{7pt}}c@{\hspace{7pt}}c@{\hspace{7pt}}c@{\hspace{7pt}}c@{\hspace{7pt}}c@{\hspace{7pt}}c@{\hspace{7pt}}c@{\hspace{7pt}}c@{\hspace{7pt}}c@{\hspace{7pt}}c@{}}
    \toprule
    Method & Mean & ATE & CM & EFF & INF & MASS & NOD & PNE & PTX & CON & EDE & EMP & FIB & PLT & HER\\
    \midrule
    GLoRIA~\cite{huang2021gloria} & 0.610 & 0.653 & 0.704 & 0.762 & 0.660 & 0.613 & 0.508 & 0.587 & 0.572 & 0.697 & 0.762 & 0.499 & 0.459 & 0.613 & 0.450 \\
    CheXzero~\cite{tiu2022expert} &  0.712 & 0.705 & 0.837 & 0.850 & 0.652 & 0.706 & 0.598 & 0.717 & 0.805 & 0.773 & 0.853 & 0.430 & 0.655 & 0.555 & 0.824 \\                                                      
    MedKLIP~\cite{wu2023medklip} & 0.726 & 0.671 & 0.842 & 0.813 & 0.706 & 0.742 & 0.621 & 0.698 & 0.821 & 0.719 & 0.803 & 0.783 & 0.604 & 0.499 &  0.841 \\
    KAD~\cite{zhang2023knowledge} & 0.789 & 0.770 & \textbf{0.854} & 0.824 & 0.694 & 0.754 & 0.698 & 0.734 & 0.860 & 0.718 & 0.809 & \textbf{0.879} & 0.780 & 0.718 & \textbf{0.952} \\
    \algname & \textbf{0.811} & \textbf{0.819} & 0.852 & \textbf{0.873} & 0.670 & \textbf{0.854} & \textbf{0.718} & \textbf{0.737} & \textbf{0.871} & \textbf{0.786} & \textbf{0.884} & 0.808 & \textbf{0.788} & \textbf{0.770} & 0.928 \\
    \bottomrule
  \end{tabular}
  \caption{Comparative analysis between the existing zero-shot classification approaches and our proposed \algname method, applied to
ChestXray14 dataset across 14 disease categories in terms of AUC performance. The abbreviations ATE, CM, EFF, INF, MASS, NOD, PNE, PTX, CON, EDE, EMP, FIB, PLT, and HER correspond to Atelectasis, Cardiomegaly, Effusion, Infiltration, Mass, Nodule, Pneumonia, Pneumothorax, Consolidation, Edema, Emphysema, Fibrosis, Pleural Thickening, and Hernia, respectively.}
  \label{tab:chexray14}
\end{table*}

\begin{table*}
  \centering
  \begin{tabular}{@{}lcccccc@{}}
    \toprule
    Method & Mean & Aelectasis &  Cardiomegaly & Consolidation & Edema & Pleural effusion\\
    \midrule
    GLoRIA~\cite{huang2021gloria} & 0.750 & 0.807 & 0.802 & 0.588 & 0.747 & 0.807\\
    CheXzero~\cite{tiu2022expert} & 0.889 & 0.816 & 0.906 & 0.892 & 0.897 & 0.932  \\
    MedKLIP~\cite{wu2023medklip}  & 0.879 & 0.813 & 0.866 & 0.858 & 0.911 & 0.947 \\
    KAD~\cite{zhang2023knowledge} & 0.905 & \textbf{0.884} & 0.885 & 0.865 & 0.943 & \textbf{0.949} \\
    \algname & \textbf{0.923} & 0.879 & \textbf{0.916} & \textbf{0.923} & \textbf{0.950} & \textbf{0.949} \\
    \bottomrule
  \end{tabular}
  \vspace{-1mm}
  \caption{Comparative analysis between the existing zero-shot classification approaches and our proposed \algname method, applied to
CheXpert dataset across 5 disease categories in terms of AUC performance.}
  \label{tab:chexpert}
  \vspace{-2mm}
\end{table*}

\begin{table*}
  \centering
  \begin{tabular}{@{}lccccccccccc@{}}
    \toprule
    Method & Mean & ATE & CALC & CONS & EFF & EMPH & FIB & FX & MASS & NOD & PTX\\
    \midrule
    GLoRIA~\cite{huang2021gloria} & 0.645 & 0.622 & 0.524 & 0.718 & 0.866 & 0.607 & 0.523 & 0.494 & 0.725 & 0.630 & 0.744\\
    CheXzero~\cite{tiu2022expert} & 0.640 & 0.622 & 0.392 & 0.826 & 0.873 & 0.503 & 0.628 & 0.665 & 0.650 & 0.479 & 0.766 \\
    MedKLIP~\cite{wu2023medklip} & 0.713 & 0.746 & 0.527 & 0.831 & 0.905 & 0.728 & 0.567 & 0.642 & 0.796 & 0.572 & 0.814  \\
    KAD~\cite{zhang2023knowledge} & 0.735 & 0.757 & 0.563 & 0.824 & 0.888 & 0.888 & 0.687 & 0.608 & 0.695 & 0.566 & 0.874 \\
    \algname &  \textbf{0.796} & \textbf{0.782} & \textbf{0.642} & \textbf{0.857} & \textbf{0.910} & \textbf{0.926} & \textbf{0.736} & \textbf{0.714} & \textbf{0.843} & \textbf{0.637} & \textbf{0.915} \\
    \bottomrule
  \end{tabular}
  \vspace{-1mm}
  \caption{Comparative analysis between the existing zero-shot classification approaches and our proposed \algname method, applied to
ChestXDet10 dataset across 10 disease categories in terms of AUC performance. The abbreviations ATE, CALC, CONS, EFF, EMPH, FIB, FX, MASS, NOD, and PTX correspond to Atelectasis, Calcification, Consolidation, Effusion, Emphysema, Fibrosis, Fracture, Mass, Nodule, and Pneumothorax, respectively.}
  \label{tab:chestxdet10}
  \vspace{-2mm}
\end{table*}

% \begin{figure*}[ht!]
%   \centering
%   % 第一行
%   \begin{subfigure}{.5\linewidth}
%     \centering
%     \includegraphics[width=\linewidth]{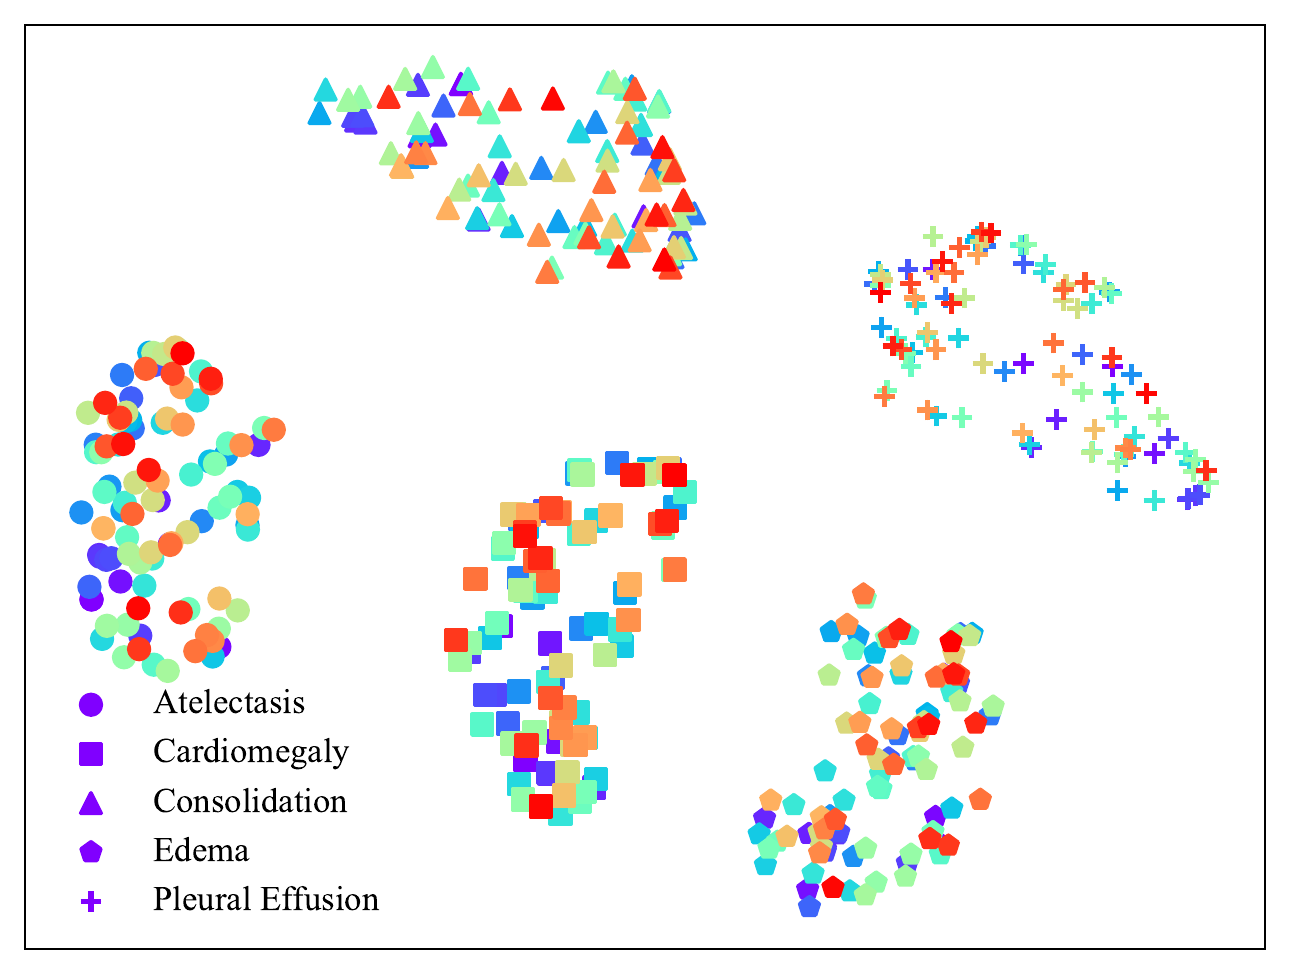}
%     \caption{First subfigure}
%     \label{fig:sub1}
%   \end{subfigure}%
%   \hfill
%   \begin{subfigure}{.5\linewidth}
%     \centering
%     \includegraphics[width=\linewidth]{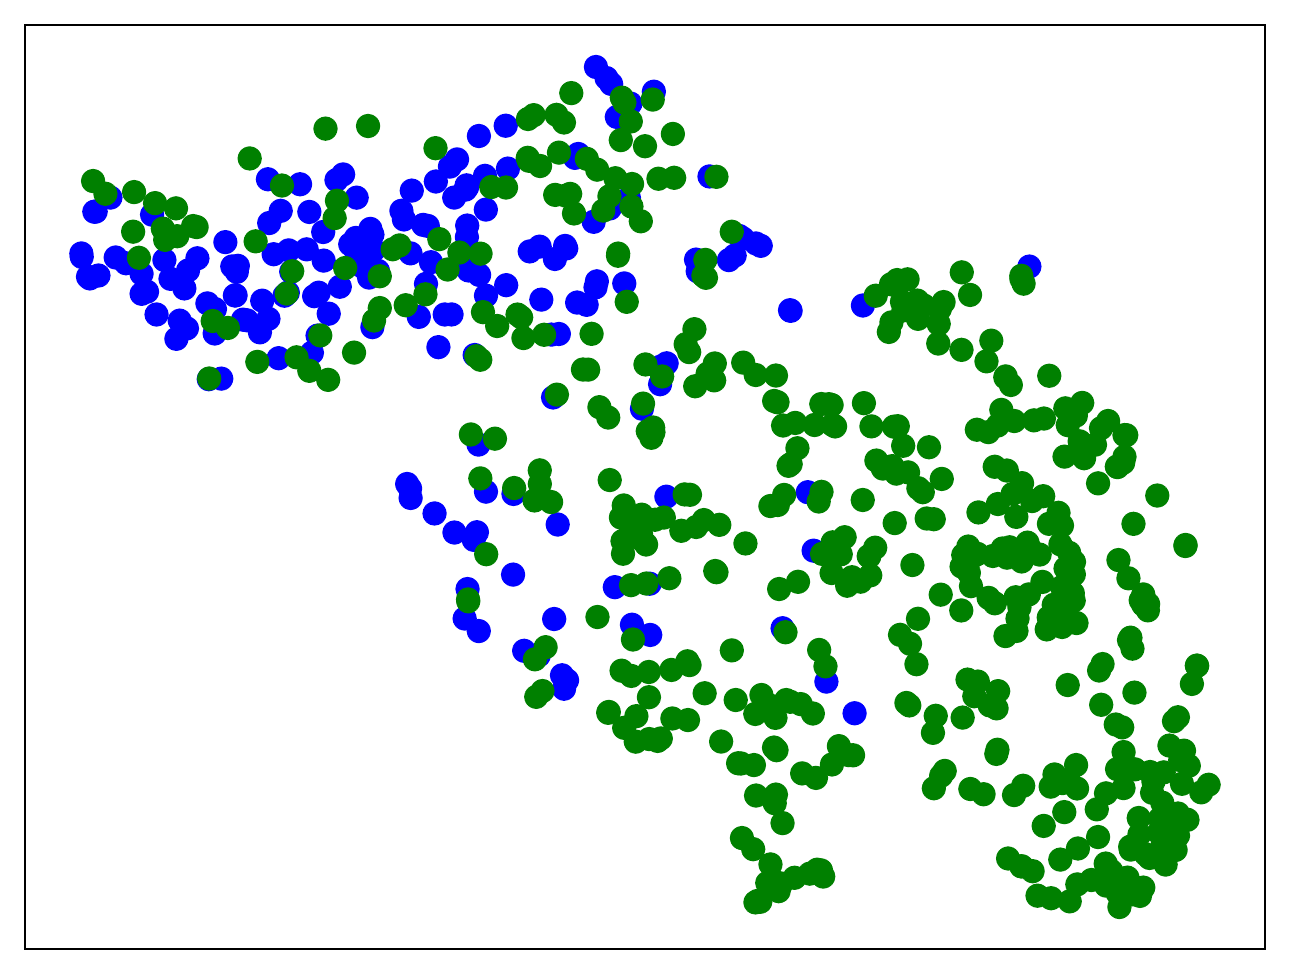}
%     \caption{Second subfigure}
%     \label{fig:sub2}
%   \end{subfigure}
%   % 第二行
%   \begin{subfigure}{.5\linewidth}
%     \centering
%     \includegraphics[width=\linewidth]{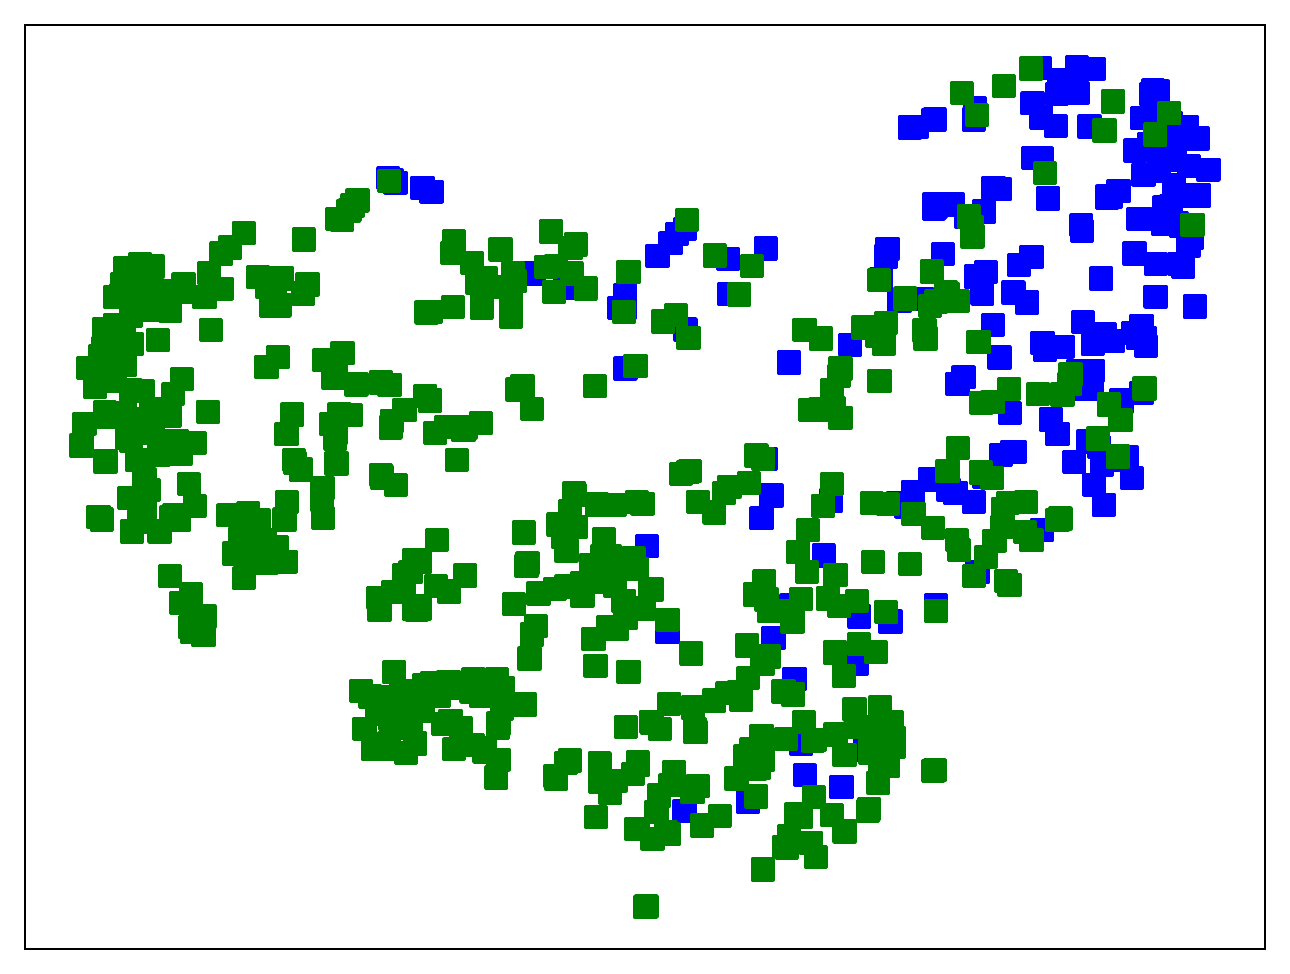}
%     \caption{Third subfigure}
%     \label{fig:sub3}
%   \end{subfigure}%
%   \hfill
%   \begin{subfigure}{.5\linewidth}
%     \centering
%     \includegraphics[width=\linewidth]{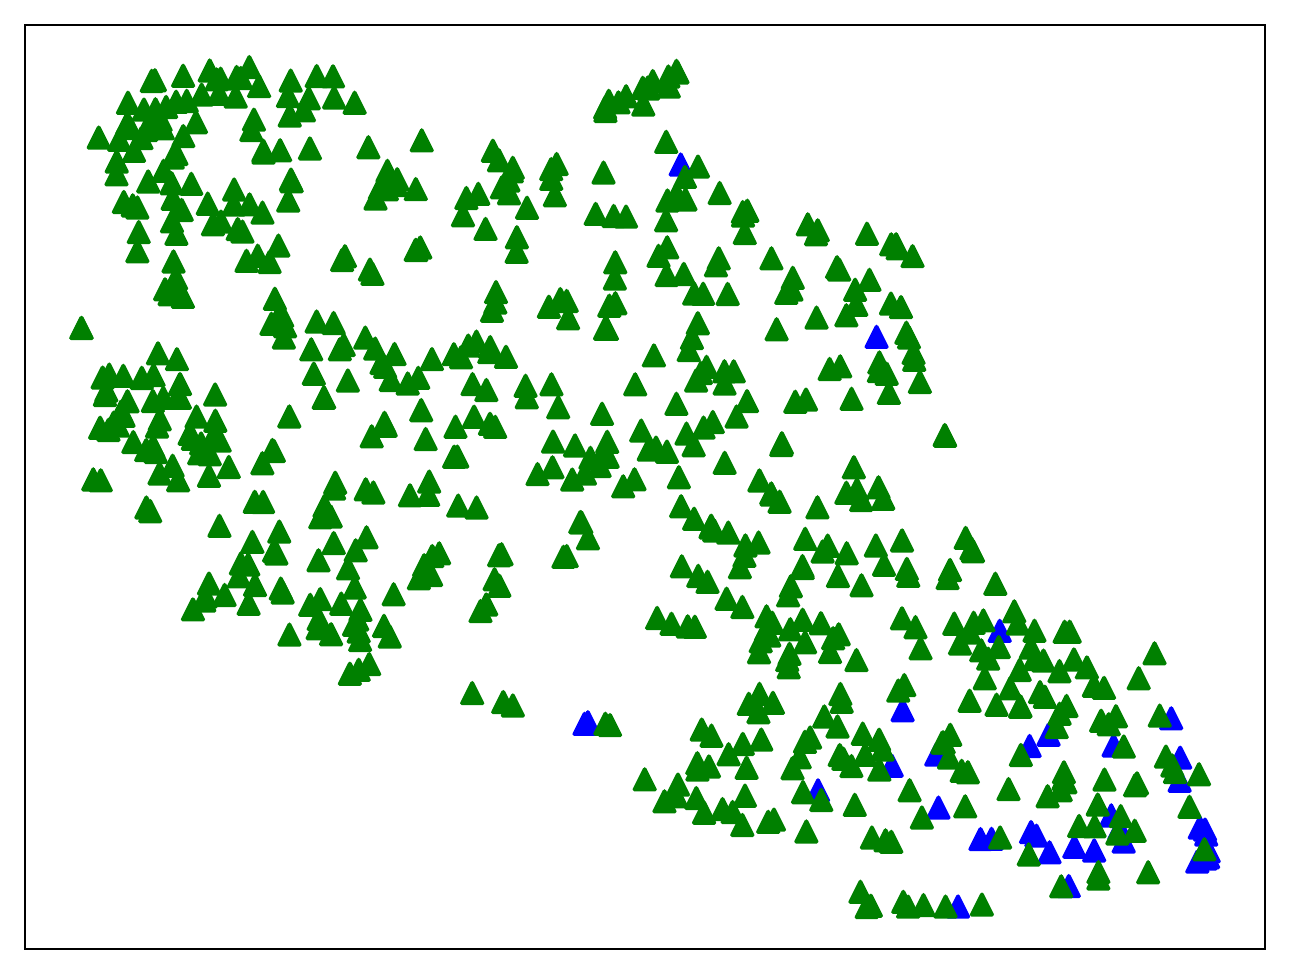}
%     \caption{Fourth subfigure}
%     \label{fig:sub4}
%   \end{subfigure}
%   % 第三行
%   \begin{subfigure}{.5\linewidth}
%     \centering
%     \includegraphics[width=\linewidth]{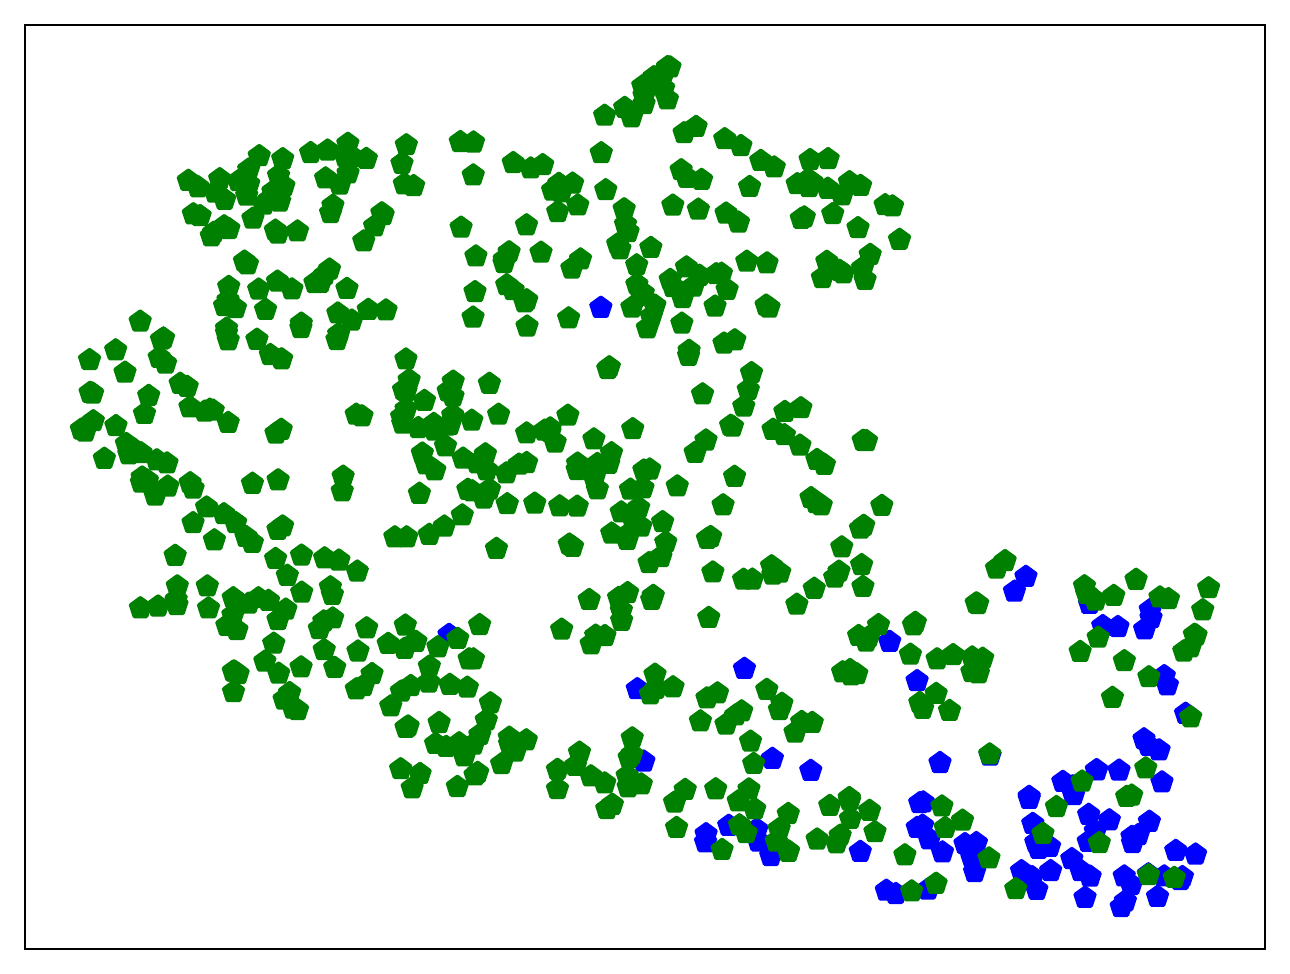}
%     \caption{Fifth subfigure}
%     \label{fig:sub5}
%   \end{subfigure}%
%   \hfill
%   \begin{subfigure}{.5\linewidth}
%     \centering
%     \includegraphics[width=\linewidth]{sec/figure/Pleural Effusion.pdf}
%     \caption{Sixth subfigure}
%     \label{fig:sub6}
%   \end{subfigure}
%   \caption{Example of a short caption for all subfigures.}
%   \label{fig:short}
% \end{figure*}

\begin{figure*}[ht!]
  \centering
  % 第一行
  \begin{subfigure}{.33\linewidth}
    \centering
    \includegraphics[width=\linewidth]{sec/figure/t_sne.pdf}
    \caption{Similarity representations}
    \label{fig:tsne:sub1}
  \end{subfigure}%
  \begin{subfigure}{.33\linewidth}
    \centering
    \includegraphics[width=\linewidth]{sec/figure/Atelectasis.pdf}
    \caption{Atelectasis}
    \label{fig:tsne:sub2}
  \end{subfigure}%
  \begin{subfigure}{.33\linewidth}
    \centering
    \includegraphics[width=\linewidth]{sec/figure/Cardiomegaly.pdf}
    \caption{Cardiomegaly}
    \label{fig:tsne:sub3}
  \end{subfigure}
  % 第二行
  \begin{subfigure}{.33\linewidth}
    \centering
    \includegraphics[width=\linewidth]{sec/figure/Consolidation.pdf}
    \caption{Consolidation}
    \label{fig:tsne:sub4}
  \end{subfigure}%
  \begin{subfigure}{.33\linewidth}
    \centering
    \includegraphics[width=\linewidth]{sec/figure/Edema.pdf}
    \caption{Edema}
    \label{fig:tsne:sub5}
  \end{subfigure}%
  \begin{subfigure}{.33\linewidth}
    \centering
    \includegraphics[width=\linewidth]{sec/figure/Pleural Effusion.pdf}
    \caption{Pleural Effusion}
    \label{fig:tsne:sub6}
  \end{subfigure}
  \caption{t-SNE visualization of similarity representations for five classes in CheXpert. (a) Different colors represent various CXRs, while distinct shapes indicate different diseases. A subset of 100 samples is randomly selected for clearer visualization. (b)-(f) display the similarity representations within each class, where blue signifies positive cases and green indicates negative cases. The total testing set of CheXpert is represented here.}
  \label{fig:tsne}

%   \newpage
% {
%     \small
%     \bibliographystyle{ieeenat_fullname}
%     \bibliography{suppl}
% }

\end{figure*}
